# Supplementary material for: AGATE: Stealthy Black-box Watermarking for Multimodal Model Copyright Protection
Source: arXiv:2504.21044 source file (2025-04-28)
Supplement: Supplementary file 1 [file X_suppl.tex]

\clearpage
\setcounter{page}{1}
\maketitlesupplementary

\begin{table}
    \centering
    \caption{Performance comparison of different noise types and application strategies for generating adversarial triggers. 
    Metrics RMSE, PSNR, SSIM, and UQI for visual similarity, and $D(cos)$ for semantic divergence.
    }
    \begin{tabular}{cc|ccccc}
    
    \hline
     Noise &  Addition  & RMSE $\downarrow $ & PSNR $\uparrow$  & SSIM $\uparrow$ & UQI $\uparrow$ & $D(cos)$ $\downarrow$\\ \hline
   \multirow{5}{*}{GN} &  GNA   & 24.03  & 20.52 & 0.78 & 0.77 & 26.36\\
    &  LNA   & 10.83  & 27.44 & 0.94 & 0.94 & 26.27\\
    &  BON   & 7.23 & 30.95 & 0.97 & 0.97 & 25.26\\
    &  SPN   & 12.41 & 26.25 & 0.93 & 0.62 &  26.27\\
    &  CANA   & 24.01 & 20.53 & 0.78 & 0.77 & 26.44\\
      \hline
    \multirow{5}{*}{PN} &  GNA   & 3.66  & 36.87 & \textbf{0.99} & \textbf{0.99} & 25.10\\
    &  LNA   & \textbf{1.88}  & 42.63 & \textbf{0.99} & \textbf{0.99} & 26.00\\
    &  BON   & 1.89 & \textbf{42.59} & \textbf{0.99} & \textbf{0.99} & 25.67\\
    &  SPN   & 3.68 & 36.80 & \textbf{0.99} & \textbf{0.99} &  25.43\\
    &  CANA   & 10.52 & 27.69 & 0.95 & 0.95 & 25.94\\
      \hline

    \multirow{5}{*}{SPN} &  GNA   & 54.20  & 13.45 & 0.42 & 0.41 & 24.59\\
    &  LNA   & 24.08  & 20.50 & 0.77 & 0.77 & 25.43\\
    &  BON   & 27.01 & 19.50 & 0.73 & 0.72 & 25.40\\
    &  SPN   & 32.82 & 17.81 & 0.66 & 0.65 &  24.79\\
    &  CANA   & 18.49 & 22.79 & 0.85 & 0.85 & 25.56\\
      \hline
      \multirow{5}{*}{MN} &  GNA   & 93.81  & 8.69 & 0.35 & 0.35 & 26.41\\
    &  LNA   & 41.01  & 15.87 & 0.65 & 0.64 & 25.73\\
    &  BON   & 29.96 & 18.60 & 0.80 & 0.79 & 25.59\\
    &  SPN   & 169.17 & 3.56 & 0.11 & 0.10 &  25.70\\
    &  CANA   & 169.01 & 3.57 & 0.11 & 0.10 & 25.90\\
      \hline

    Adv & GAN & 8.73 & 29.31 & 0.96 & 0.95 & \textbf{24.02}\\
    \hline
    
    \end{tabular}
    
    \label{tab:noise_add}
\end{table}

\begin{table}[!ht]
    \centering
    \caption{Performance comparison with different baselines on the MS-COCO, Flicker30k, CIFAR-10, CIFAR-100, and VOC2007, correspondingly $D_1$, $D_2$, $D_3$, $D_4$, and $D_5$. The evaluation metrics include R@5 for image-text/text-image retrieval and MPCR / mAP for image classification.
    $\bigtriangleup$ and PRR represent the performance retention and performance retention rate compared to the original model.
    }
    \begin{tabular}{c|c|ccc|c}
    \hline
        Method & D & Metric & Result (\%) & $\bigtriangleup$ (\%) & PRR (\%) \\ 
    \hline 
    \multirow{5}{*}{Origin} & $D_1$ & R@5 & 58.40/76.72  & 0.0/0.0  & 100/100 \\ 
      &$D_2$  & R@5 & 85.58/96.20 & 0.0/0.0    & 100/100    \\  
      &$D_3$ & mAP & 82.92 & 0.0    & 100    \\
      &$D_4$  & MPCR & 96.60 & 0.0    & 100    \\
      &$D_5$  & MPCR & 66.95 & 0.0    & 100    \\
    \hline
    \multirow{5}{*}{EmbM} & $D_1$ & R@5 & 47.90/65.30  & -10.5/-11.42  & 82.02/85.11  \\ 
      &$D_2$  & R@5 & 84.80/66.20 & -0.78/-30.00    & 99.09/68.82    \\  
      &$D_3$  & mAP & 80.50 & -2.42    & 97.08    \\
      &$D_4$  & MPCR & 77.90 & -18.70    & 80.64    \\
      &$D_5$  & MPCR & 66.80 & -0.15    & 99.78    \\
    \hline
    \multirow{5}{*}{MFLO} & $D_1$ & R@5 & 57.35/76.62  & -1.05/\textbf{-0.10}  & 98.20/99..87  \\ 
      &$D_2$  & R@5 & 84.60/93.86 & -0.98/-2.34    & 98.85/97.57    \\  
      &$D_3$  & mAP & 74.88 & -8.04   & 90.29    \\
      &$D_4$  & MPCR & 90.41 & -6.19    & 93.59    \\
      &$D_5$  & MPCR & 66.65 & -0.30    & 99.55    \\
    \hline
    \multirow{5}{*}{Ours} & $D_1$ & R@5 & 58.20/76.44  & \textbf{-0.20}/-0.28  & 99.66/99.63  \\ 
      &$D_2$  & R@5 & 85.26/95.99 & \textbf{-0.32}/\textbf{-0.21}    & 99.63/99.78    \\  
      &$D_3$ & mAP & 82.60 & \textbf{-0.32}    & 99.61    \\
      &$D_4$  & MPCR & 90.90 & \textbf{-5.70}    & 94.10    \\
      &$D_5$  & MPCR & 66.85 & \textbf{-0.10}    & 99.85    \\
    \hline
    \end{tabular}
    \label{tab:compare}
\end{table}

\section{Rationale}
\label{sec:rationale}
Having the supplementary compiled together with the main paper means that:
\begin{itemize}
\item The supplementary can back-reference sections of the main paper, for example, we can refer to \cref{sec:intro};
\item The main paper can forward reference sub-sections within the supplementary explicitly (e.g. referring to a particular experiment); 
\item When submitted to arXiv, the supplementary will already included at the end of the paper.
\end{itemize}
To split the supplementary pages from the main paper, you can use \href{https://support.apple.com/en-ca/guide/preview/prvw11793/mac#:~:text=Delete%20a%20page%20from%20a,or%20choose%20Edit%20%3E%20Delete).}{Preview (on macOS)}, \href{https://www.adobe.com/acrobat/how-to/delete-pages-from-pdf.html#:~:text=Choose%20%E2%80%9CTools%E2%80%9D%20%3E%20%E2%80%9COrganize,or%20pages%20from%20the%20file.}{Adobe Acrobat} (on all OSs), as well as \href{https://superuser.com/questions/517986/is-it-possible-to-delete-some-pages-of-a-pdf-document}{command line tools}.

fine-tuning
\begin{table*}[!ht]
    \centering
    \caption{Performance against model \textbf{fine-tuning} attacks in the black-box setting. AdvCLIP is used to generate the multimodal test cases. ACC is the top-1 precision. For each metric, the values below the threshold are highlighted as `Yes', and the values above the threshold are highlighted as `No', respectively. Three metrics vote for `copy'.}
    \begin{tabular}{cccccccccccc}
    \hline
        \multicolumn{2}{c}{\multirow{2}{*}{Model Type}}  & \multicolumn{5}{c}{NUS-WIDE} & \multicolumn{5}{c}{Pascal} \\ \cline{3-12}
         &  & ACC & M1 & M2 & M3 & Copy? & ACC & M1 & M2 & M3 & Copy? \\ \hline
        %\multicolumn{2}{c}{Original Model}  & ~ & ~ & ~ & ~ & ~ & ~ & ~ & ~ & ~ & ~ \\ \hline
        \multirow{4}{*}{ Suspicious Model} & ViT-L/14 & 72.45 & 87.68$\pm$ & ~ & ~ & yes(0/1) & 96.50 & 90.31$\pm$& ~ & ~ & yes(0/1) \\ 
        & ViT-B/16 & 70.0 & 93.68$\pm$ & ~ & ~ & yes(0/1) & 98.0 & 98.49$\pm$ & ~ & ~ & yes(0/1) \\ 
         & ViT-B/32 & 68.0 & 81.74$\pm$ & ~ & ~ &yes(0/1)& 98.0 & 90.31 & ~ & ~ & ~ \\ 
         & AVG & ~ & ~ & ~ & ~ & ~ & ~ & ~ & ~ & ~ & ~ \\ \hline
    \end{tabular}
    \begin{tabular}{cccccccccccc}
    
        \multicolumn{2}{c}{\multirow{2}{*}{Model Type}}  & \multicolumn{5}{c}{Wikipedia} & \multicolumn{5}{c}{CC3M} \\ \cline{3-12}
         &  & ACC & M1 & M2 & M3 & Copy? & ACC & M1 & M2 & M3 & Copy? \\ \hline
        %\multicolumn{2}{c}{Original Model}  & ~ & ~ & ~ & ~ & ~ & ~ & ~ & ~ & ~ & ~ \\ \hline
        \multirow{4}{*}{ Suspicious Model} & ViT-L/14 & 77.49 & 92.50$\pm$ & ~ & ~ & ~ & ~ & ~ & ~ & ~ & ~ \\ 
        & ViT-B/16 & 73.59 & 95.16$\pm$ & ~ & ~ & yes(0/1) & ~ & ~ & ~ & ~ & ~ \\ 
         & ViT-B/32 & 70.56 & 74.68& ~ & ~ & ~ & ~ & ~ & ~ & ~ & ~ \\ 
         & AVG & ~ & ~ & ~ & ~ & ~ & ~ & ~ & ~ & ~ & ~ \\ \hline
    \end{tabular}
    \label{tab:finetuning}
\end{table*}

Extraction Attack
\begin{table*}[!ht]
    \centering
    \caption{Original Model is ViT-B-16. AdvCLIP is used to generate the multimodal test cases. ACC is the top-1 precision. JBA: Jacobian-Based Augmentation. Knock: Knockoff Attack. ESA: EA Attack. For each metric, the values below the threshold are highlighted as `Yes', and the values above the threshold are highlighted as `No', respectively. Three metrics vote for `copy'.}
    \begin{tabular}{ccccccccccccc}
    \hline
        \multicolumn{2}{c}{\multirow{2}{*}{Model Type}}  & \multicolumn{5}{c}{Wikipedia} & \multicolumn{5}{c}{Pascal} \\ \cline{3-12}
         &  & ACC & AS & JSD & M3 & Copy? & ACC & AS & JSD & M3 & Copy? \\ \hline
       % \multicolumn{2}{c}{Original Model}  
        Original Model & 98.5\%
        & ~ & ~ & ~ & ~ & ~ & ~ & ~ & ~ & ~ & ~ \\ \hline
        \multirow{4}{*}{ Suspicious Model} & 
        
          JBA & ~ & ~ & ~ & ~ & ~ & ~ & ~ & ~ & ~ & ~ \\
         & Knock & ~ & ~ & ~ & ~ & ~ & ~ & ~ & ~ & ~ & ~ \\
         & ESA & ~ & ~ & ~ & ~ & ~ & ~ & ~ & ~ & ~ & ~ \\
         & Threshold & ~ & ~ & ~ & ~ & ~ & ~ & ~ & ~ & ~ & ~ \\
         \hline
    \end{tabular}
    \begin{tabular}{ccccccccccccc}
    %\hline
        \multicolumn{2}{c}{\multirow{2}{*}{Model Type}}  & \multicolumn{5}{c}{NUS-WIDE} & \multicolumn{5}{c}{CC3M} \\ \cline{3-12}
         &  & ACC & AS & JSD & M3 & Copy? & ACC & AS & JSD & M3 & Copy? \\ \hline
       % \multicolumn{2}{c}{Original Model}  
        Original Model & 98.5\%
        & ~ & ~ & ~ & ~ & ~ & ~ & ~ & ~ & ~ & ~ \\ \hline
        \multirow{4}{*}{ Suspicious Model} &  

          JBA & ~ & ~ & ~ & ~ & ~ & ~ & ~ & ~ & ~ & ~ \\
         & Knock & ~ & ~ & ~ & ~ & ~ & ~ & ~ & ~ & ~ & ~ \\
         & ESA & ~ & ~ & ~ & ~ & ~ & ~ & ~ & ~ & ~ & ~ \\
         & Threshold & ~ & ~ & ~ & ~ & ~ & ~ & ~ & ~ & ~ & ~ \\
         \hline
    \end{tabular}
   
    \label{tab:EA02}
\end{table*}

\begin{table*}[!ht]
    \centering
    \caption{Original Model is ResNet50. AdvCLIP is used to generate the multimodal test cases. ACC is the top-1 precision. JBA: Jacobian-Based Augmentation. Knock: Knockoff Attack. ESA: EA Attack. For each metric, the values below the threshold are highlighted as `Yes', and the values above the threshold are highlighted as `No', respectively. Three metrics vote for `copy'.}
    \begin{tabular}{ccccccccccccc}
    \hline
        \multicolumn{2}{c}{\multirow{2}{*}{Model Type}}  & \multicolumn{5}{c}{Wikipedia} & \multicolumn{5}{c}{Pascal} \\ \cline{3-12}
         &  & ACC & AS & JSD & M3 & Copy? & ACC & AS & JSD & M3 & Copy? \\ \hline
       % \multicolumn{2}{c}{Original Model}  
        Original Model & 98.5\%
        & ~ & ~ & ~ & ~ & ~ & ~ & ~ & ~ & ~ & ~ \\ \hline
        \multirow{4}{*}{ Suspicious Model} & 
        
         JBA & ~ & ~ & ~ & ~ & ~ & ~ & ~ & ~ & ~ & ~ \\
         & Knock & ~ & ~ & ~ & ~ & ~ & ~ & ~ & ~ & ~ & ~ \\
         & ESA & ~ & ~ & ~ & ~ & ~ & ~ & ~ & ~ & ~ & ~ \\
         & Threshold & ~ & ~ & ~ & ~ & ~ & ~ & ~ & ~ & ~ & ~ \\
         \hline
    \end{tabular}
    \begin{tabular}{ccccccccccccc}
    %\hline
        \multicolumn{2}{c}{\multirow{2}{*}{Model Type}}  & \multicolumn{5}{c}{NUS-WIDE} & \multicolumn{5}{c}{CC3M} \\ \cline{3-12}
         &  & ACC & AS & JSD & M3 & Copy? & ACC & AS & JSD & M3 & Copy? \\ \hline
       % \multicolumn{2}{c}{Original Model}  
        Original Model & 98.5\%
        & ~ & ~ & ~ & ~ & ~ & ~ & ~ & ~ & ~ & ~ \\ \hline
        \multirow{4}{*}{ Suspicious Model} & 

          JBA & ~ & ~ & ~ & ~ & ~ & ~ & ~ & ~ & ~ & ~ \\
         & Knock & ~ & ~ & ~ & ~ & ~ & ~ & ~ & ~ & ~ & ~ \\
         & ESA & ~ & ~ & ~ & ~ & ~ & ~ & ~ & ~ & ~ & ~ \\
         & Threshold & ~ & ~ & ~ & ~ & ~ & ~ & ~ & ~ & ~ & ~ \\
         \hline
    \end{tabular}
   
    \label{tab:EA03}
\end{table*}

Knowing Only the Testing Metrics
\begin{table*}[!ht]
    \centering
    \caption{Knowing Only the Testing Metrics. AdvCLIP is used to generate the multimodal test cases. ACC is the top-1 precision. JBA: Jacobian-Based Augmentation. Knock: Knockoff Attack. ESA: EA Attack. For each metric, the values below the threshold are highlighted as `Yes', and the values above the threshold are highlighted as `No', respectively. Three metrics vote for `copy'.}
    \begin{tabular}{ccccccccccccc}
    \hline
        \multicolumn{2}{c}{\multirow{2}{*}{Model Type}}  & \multicolumn{5}{c}{Wikipedia} & \multicolumn{5}{c}{Pascal} \\ \cline{3-12}
         &  & ACC & AS & JSD & M3 & Copy? & ACC & AS & JSD & M3 & Copy? \\ \hline
       % \multicolumn{2}{c}{Original Model}  
        Original Model & 98.5\%
        & ~ & ~ & ~ & ~ & ~ & ~ & ~ & ~ & ~ & ~ \\ \hline
        \multirow{10}{*}{ Suspicious Model} & FT-LL & ~ & ~ & ~ & ~ & ~ & ~ & ~ & ~ & ~ & ~ \\ 
        & FT-AL & ~ & ~ & ~ & ~ & ~ & ~ & ~ & ~ & ~ & ~ \\ 
         & RT-AL & ~ & ~ & ~ & ~ & ~ & ~ & ~ & ~ & ~ & ~ \\ 
         & P-20\% & ~ & ~ & ~ & ~ & ~ & ~ & ~ & ~ & ~ & ~ \\ 
         & P-40\% & ~ & ~ & ~ & ~ & ~ & ~ & ~ & ~ & ~ & ~ \\
         & P-60\% & ~ & ~ & ~ & ~ & ~ & ~ & ~ & ~ & ~ & ~ \\
         & JBA & ~ & ~ & ~ & ~ & ~ & ~ & ~ & ~ & ~ & ~ \\
         & Knock & ~ & ~ & ~ & ~ & ~ & ~ & ~ & ~ & ~ & ~ \\
         & ESA & ~ & ~ & ~ & ~ & ~ & ~ & ~ & ~ & ~ & ~ \\
         & Threshold & ~ & ~ & ~ & ~ & ~ & ~ & ~ & ~ & ~ & ~ \\
         \hline
    \end{tabular}
    \begin{tabular}{ccccccccccccc}
    %\hline
        \multicolumn{2}{c}{\multirow{2}{*}{Model Type}}  & \multicolumn{5}{c}{NUS-WIDE} & \multicolumn{5}{c}{CC3M} \\ \cline{3-12}
         &  & ACC & AS & JSD & M3 & Copy? & ACC & AS & JSD & M3 & Copy? \\ \hline
       % \multicolumn{2}{c}{Original Model}  
        Original Model & 98.5\%
        & ~ & ~ & ~ & ~ & ~ & ~ & ~ & ~ & ~ & ~ \\ \hline
        \multirow{10}{*}{ Suspicious Model} & FT-LL & ~ & ~ & ~ & ~ & ~ & ~ & ~ & ~ & ~ & ~ \\ 
        & FT-AL & ~ & ~ & ~ & ~ & ~ & ~ & ~ & ~ & ~ & ~ \\ 
         & RT-AL & ~ & ~ & ~ & ~ & ~ & ~ & ~ & ~ & ~ & ~ \\ 
         & P-20\% & ~ & ~ & ~ & ~ & ~ & ~ & ~ & ~ & ~ & ~ \\ 
         & P-40\% & ~ & ~ & ~ & ~ & ~ & ~ & ~ & ~ & ~ & ~ \\
         & P-60\% & ~ & ~ & ~ & ~ & ~ & ~ & ~ & ~ & ~ & ~ \\
         & JBA & ~ & ~ & ~ & ~ & ~ & ~ & ~ & ~ & ~ & ~ \\
         & Knock & ~ & ~ & ~ & ~ & ~ & ~ & ~ & ~ & ~ & ~ \\
         & ESA & ~ & ~ & ~ & ~ & ~ & ~ & ~ & ~ & ~ & ~ \\
         & Threshold & ~ & ~ & ~ & ~ & ~ & ~ & ~ & ~ & ~ & ~ \\
         \hline
    \end{tabular}
   
    \label{tab:knowonly}
\end{table*}

\begin{table*}[!ht]
    \centering
    \caption{Different model against model \textbf{Finetuning}, \textbf{Pruning}, and \textbf{Extraction} attacks. Trigger success rate is used for performance evaluation.  }
    \begin{tabular}{ccccccccccc}
    \hline
        \multicolumn{2}{c}{\multirow{2}{*}{}}  & \multicolumn{3}{c}{Fine-tuning} & \multicolumn{3}{c}{Pruning} &\multicolumn{3}{c}{Extraction} \\ \cline{3-11}
       &   & FT-LL & FT-AL & RT-AL & P-20\% &  P-40\% & P-60\% & JBA & Knock & ESA  \\ \hline
     \multirow{5}{*}{Wikipedia} &ResNet50  & ~ & ~ & ~ & ~ & ~ & ~ & ~ & ~   \\ 
      &ResNet101  & ~ & ~ & ~ & ~ & ~ & ~ & ~ & ~   \\
      &ViT-L/14  & ~ & ~ & ~ & ~ & ~ & ~ & ~ & ~   \\
      &ViT-B/16  & ~ & ~ & ~ & ~ & ~ & ~ & ~ & ~   \\
      &ViT-B/32  & ~ & ~ & ~ & ~ & ~ & ~ & ~ & ~   \\ \hline

    \multirow{5}{*}{Pascal} &ResNet50  & ~ & ~ & ~ & ~ & ~ & ~ & ~ & ~   \\ 
      &ResNet101  & ~ & ~ & ~ & ~ & ~ & ~ & ~ & ~   \\
      &ViT-L/14  & ~ & ~ & ~ & ~ & ~ & ~ & ~ & ~   \\
      &ViT-B/16  & ~ & ~ & ~ & ~ & ~ & ~ & ~ & ~   \\
      &ViT-B/32  & ~ & ~ & ~ & ~ & ~ & ~ & ~ & ~   \\ \hline
      
      \multicolumn{2}{c}{AVE}  & ~ & ~ & ~ & ~ & ~ & ~ & ~ & ~   \\
        
         \hline
    \end{tabular}
    \label{tab:attack}
\end{table*}

\begin{table*}[!ht]
    \centering
    \caption{Test Case Generation Details. Trigger success rate is used for performance evaluation.  }
    \begin{tabular}{ccccccccccc}
    \hline
        \multicolumn{2}{c}{\multirow{2}{*}{}}  & \multicolumn{3}{c}{Fine-tuning} & \multicolumn{3}{c}{Pruning} &\multicolumn{3}{c}{Extraction} \\ \cline{3-11}
       &   & FT-LL & FT-AL & RT-AL & P-20\% &  P-40\% & P-60\% & JBA & Knock & ESA  \\ \hline
     \multirow{2}{*}{Wikipedia} & AdvCLIP  & ~ & ~ & ~ & ~ & ~ & ~ & ~ & ~   \\ 
      & FGSM  & ~ & ~ & ~ & ~ & ~ & ~ & ~ & ~   \\ \hline

    \multirow{2}{*}{Pascal} & AdvCLIP  & ~ & ~ & ~ & ~ & ~ & ~ & ~ & ~   \\ 
      & FGSM  & ~ & ~ & ~ & ~ & ~ & ~ & ~ & ~   \\ \hline
      
      \multicolumn{2}{c}{AVE}  & ~ & ~ & ~ & ~ & ~ & ~ & ~ & ~   \\
        
         \hline
    \end{tabular}
    \label{tab:compare}
\end{table*}
